# Supplementary material for: FlexNN: A Dataflow-aware Flexible Deep Learning Accelerator for Energy-Efficient Edge Devices
Source: arXiv:2403.09026 source file (2024-04-11)
Supplement: Supplementary file 1 [file 8_appendix.tex]

 % FSAD REVISED LOAD

%  iii.	Use Case: Tensor Data Distribution in ResNet101 Convolution Layers Using FSAD 
% We provide a use case in this session to show the operation of FSAD Unit for flexible schedules. We first show the mismatch challenges between 2 different schedules, and then present the solutions using our proposed design. We assume 16x16 PE arrays with 16 SRAM banks and 16 SRAM buffers in the following description (N=16). Note our proposal is still valid for other PE array dimensions.
% 1)	Schedule Mismatch Example in 2 Consecutive Layers in ResNet101:
% Fig. 7 (a) and (b) illustrate 2 different optimal schedules for 2 different layers of ResNet101 mapping to a 16x16 PE array, respectively. For scale3a_branch2c, its optimal schedule maps 16 partitions of 8 Oc and 16 partitions of 8 Ic to 16 rows and 16 columns of the PE array, respectively. Each PE takes 8 input channel (Ic) points and 8 output channel (Oc) points to generate 64 OF points. Therefore, it requires 8 IF points for 8 different Ic, and 64 FL points for 8 different Ic and 8 different Oc. 28 Ox, 28 Oy as well as the remaining 4 partitions of Oc are in the outer loops. Since 16 partitions of Ic map to 16 columns, the final OF requires accumulation along the PE row direction (e.g. PE(i, 15) for i=0 to 15), and the OF extraction is from the last PE column. Since FL is reused by outer loop Oy and Ox, this dataflow is weight stationary.
 
% Fig. 8. (New) Illustration of (a) optimal schedule mapping and (b) OF volume generation of scale3a_branch2c, (c) optimal schedule mapping and (d) IF volume generation of res3b1_branch2a.

% Different from scale3a_branch2c, res3b1_branch2a’s optimal schedule requires 16 partitions of 8 Oc, 14 partitions of 2 Oy and 1 partition of 4 Ox mapping to the 16x16 PE array, where Oy and Oc mapping to 16 rows and 16 columns, respectively. Therefore, it requires 8 IF points for 4 different Ox and 2 different Oy, and 8 FL points for 8 different Oc. Each PE will generate 64 Psums of 1 Ic. Since 512 partitions of Ic and 7 partitions of Ox are in the outer loops, 64 OF points per PE for 256 PEs are generated after 512 outer loops (Fig. 7(b)). Since IF and FL are brought to PEs every inner loop and Psum is stationary across all PEs, this dataflow is output stationary. Note that in Resnet101, although res3b1_branch2a and scale3a_branch2c has element-wise operation layer in-between, the data pattern mismatch remains.

% Fig. 8 (a) and (b) further show the scale3a_branch2c generated OF volume. In terms of Ox x Oy x Oc, 1x1x8 OF volume is generated per PE, and in total 1x1x128 OF volume is generated from entire PE array per inner loop block. For 28 Oy outer blocks, the OF volume is filled in the order of Outer Loop #1, #2, …, #28 for Oy=0,1,2, …, 27 at the same Ox point (e.g. Ox=0), respectively. After filling 1x28x128 OF volume for Ox=0, another 1x28x128 OF volume starts to fill for Ox=1, 2,…,27, until the entire output tensor data is generated.

% Fig.8 (c) and (d) show the IF data pattern that is required of the next layer res3b1_branch2a. Note the OF volume generated by scale3a_branch2c (shown Fig. 8 (b)) is the IF volume for this layer. Since 14 partitions Oy map to 14 PE rows, 16 partitions of Oc map to 16 PE columns, each PE requires 8 IF points, namely, 4 Ix and 2 different Iy of the same Ic. Comparing Fig. 8 (b) with Fig. 8 (d), a clear mismatch between OF of scale3a_branch2c and IF of res3b1_branch2a can be observed due to the schedule differences. Direct feed the OF volume from scale3a_branch2c to res3b1_branch2a will encounter 
